# Supplementary material for: Deep Perm-Set Net: Learn to predict sets with unknown permutation and cardinality using deep neural networks
Source: arXiv:1805.00613 source file (2018-10-02)
Supplement: Supplementary file 1 [file ref-appendix.tex]

@inproceedings{rezatofighi2018joint0,
	title={Joint learning of set cardinality and state distribution},
	author={Rezatofighi, Seyed Hamid and Milan, Anton and Shi, Qinfeng and Dick, Anthony and Reid, Ian},
	booktitle={{AAAI}},
	year={2018}
}
